# Supplementary material for: Existence of spiral strategies for blocking fire spreading
Source: arXiv:2508.05324 source file (2025-08-07)
Supplement: Supplementary file 1 [file appendix.tex]

\section{Appendix}
\label{S:appendix: fire}
Here the code provides the evaluation of the relevant quantities related to the function $\bar f_s$, computed explicitly in the previous section: we do not ask the program to solve any PDE or ODE. The evaluation of these functions are hard to perform by hand, and even if we do a careful analysis (like the study of minima and maxima of the functions), at some point one needs to use a calculator. 

\subsection{Numerical Computations for the Arc Case}\label{s:appendix:arc} In this section we present the numerical computations for the arc case (see Chapter \ref{c:family}, Section \ref{S:arc}). The orange line represents $y=0$
\begin{figure}[H]
    \centering \includegraphics{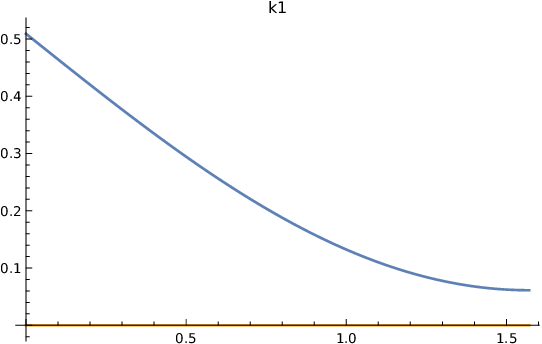}
     \caption{Computations for the arc case: $\kappa_1$.}
     \label{fig:arc:k:1}
\end{figure}

\begin{figure}[H]
    \centering 
    \includegraphics{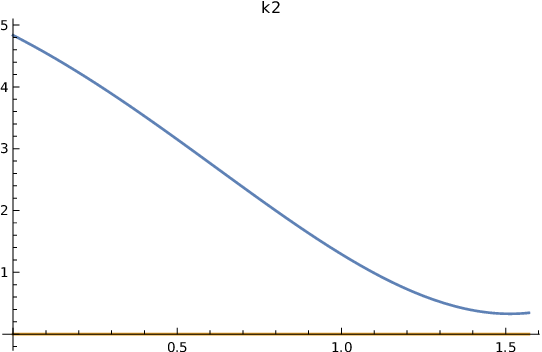}
    \caption{Computations for the arc case: $\kappa_2$.}
    \label{fig:arc:k:2}
\end{figure}
\begin{figure}[H]
    \centering \includegraphics{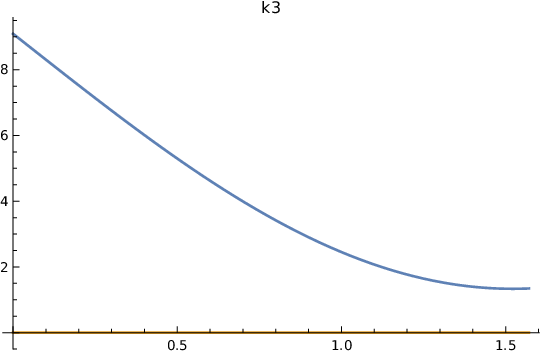}
     \caption{Computations for the arc case: $\kappa_3$.}
     \label{fig:arc:k:3}
\end{figure}
\begin{figure}[H]
    \centering \includegraphics{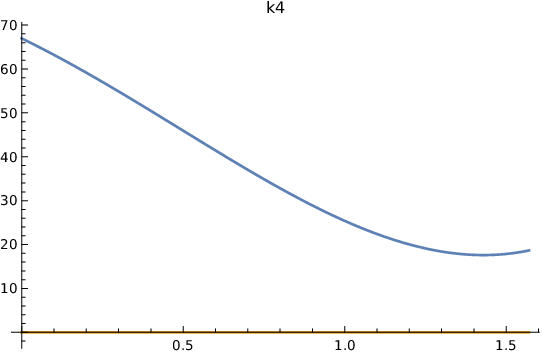}
     \caption{Computations for the arc case: $\kappa_4$.}
     \label{fig:arc:k:4}
\end{figure}
\begin{figure}[H]
    \centering \includegraphics{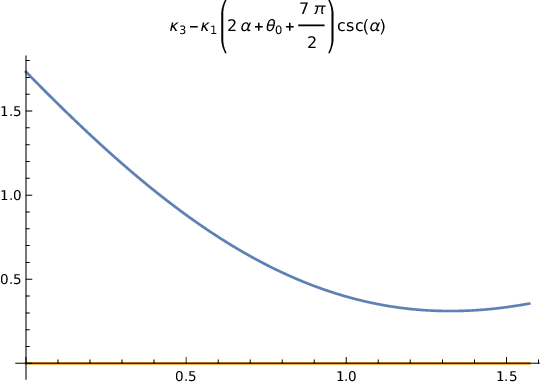}
     \caption{Computations for the arc case: $\kappa_3-\frac{\kappa_1}{\sin\alpha}\left(2\alpha+\theta_0+7\frac{\pi}{2}\right)$.}
     \label{fig:arc:Q:1}
\end{figure}
\begin{figure}[H]
    \centering \includegraphics{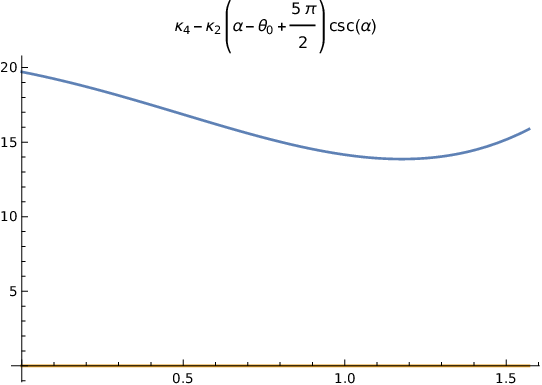}
    \caption{Computations for the arc case: $\kappa_4-\frac{\kappa_2}{\sin\alpha}\left(\alpha-\theta_0+5\frac{\pi}{2}\right)$.}
    \label{fig:arc:Q:2}
\end{figure}

\newpage
\subsection{Numerical Computations for the Segment Case}\label{s:appendix:segm} In this section we present the numerical computations for the segment case (see Chapter \ref{c:family}, Section \ref{S:segment}). The blue plane corresponds to $z=0$.

\begin{figure}[H]
    \centering \includegraphics[scale=0.6]{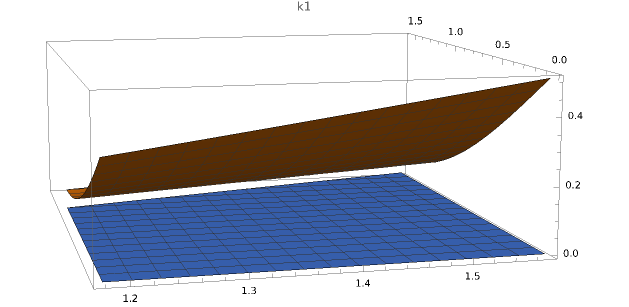}
     \caption{Computations for the segment case: $\kappa_1$.}
     \label{fig:seg:k:1}
\end{figure}
\begin{figure}[H]
    \centering 
    \includegraphics[scale=0.5]{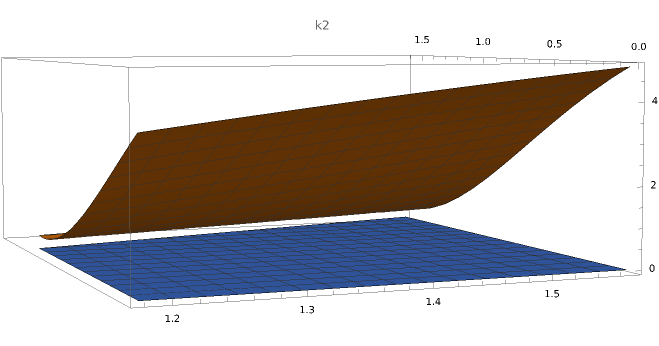}
    \caption{Computations for the segment case: $\kappa_2$.}
    \label{fig:seg:k:2}
\end{figure}
\begin{figure}[H]
    \centering \includegraphics[scale=0.6]{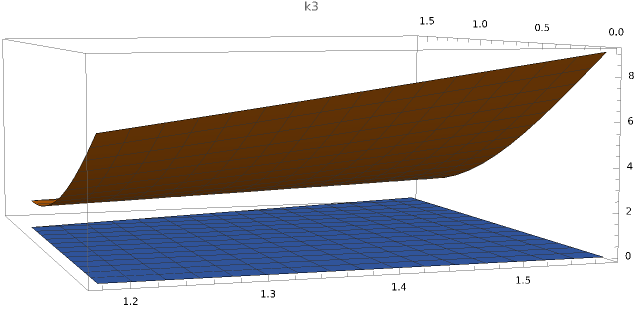}
     \caption{Computations for the segment case: $\kappa_3$.}
     \label{fig:seg:k:3}
\end{figure}
\begin{figure}[H]
    \centering \includegraphics[scale=0.7]{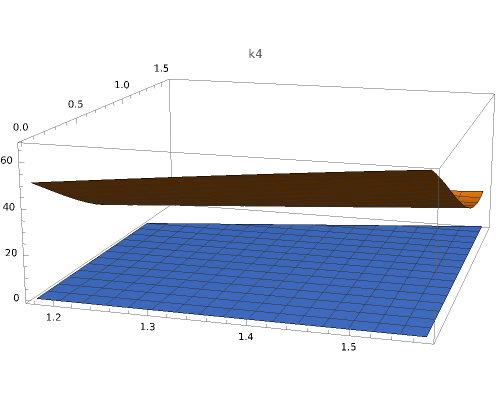}
     \caption{Computations for the segment case: $\kappa_4$.}
     \label{fig:seg:k:4}
\end{figure}
\begin{figure}[H]
    \centering \includegraphics[scale=0.7]{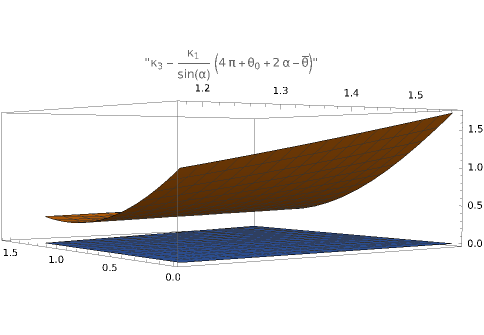}
     \caption{Computations for the segment case: $\kappa_3-\frac{\kappa_1}{\sin\alpha}\left(4\pi+2\alpha+\theta_0-\bar\theta\right)$.}
     \label{fig:seg:Q:1}
\end{figure}
\begin{figure}[H]
    \centering \includegraphics[scale=0.7]{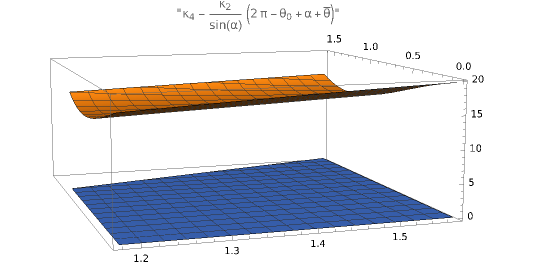}
    \caption{Computations for the segment case: $\kappa_4-\frac{\kappa_2}{\sin\alpha}\left(2\pi+\alpha-\theta_0+\bar\theta\right)$.}
     \label{fig:seg:Q:2}
\end{figure}
